# Supplementary material for: Quasiparticle Mass Enhancement and Temperature Dependence of the Electronic Structure of Ferromagnetic SrRuO3 Thin Films
Source: arXiv:1211.2828 source file (2013-03-11)
Supplement: Supplementary file 1 [file SrRuO3_Supplemental.pdf]

# Supplemental Information:
# Quasiparticle Mass Enhancement and Temperature Dependence of the Electronic Structure of Ferromagnetic $SrRuO_3$ Thin Films

D.E. Shai,[1] C. Adamo,[2] D.W. Shen,[1,2,3] C.M. Brooks,[2,4] J.W. Harter,[1]
E.J. Monkman,[1] B. Burganov,[1] D.G. Schlom,[2,5] and K.M. Shen[1,5,*]

[1]*Laboratory of Atomic and Solid State Physics, Department of Physics, Cornell University, Ithaca, New York 14853, USA*
[2]*Department of Materials Science and Engineering, Cornell University, Ithaca, New York 14853, USA*
[3]*Superconductor Applications State Key Laboratory of Functional Materials for Informatics, Chinese Academy of Sciences, Shanghai 200050, China*
[4]*Department of Materials Science and Engineering, The Pennsylvania State University, University Park, Pennsylvania 16802, USA*
[5]*Kavli Institute at Cornell for Nanoscale Science, Ithaca, New York 14853, USA*

## FILM GROWTH AND RHEED CHARACTERIZATION

20 nm thick films of $(001)_p$ $SrRuO_3$ (where the subscript $p$ denotes pseudocubic indices) were deposited epitaxially on $(001)_p$ $NdGaO_3$ single crystal substrates in a Veeco GEN10 dual-chamber oxide MBE. During growth the substrate was held at 800 °C and the oxidant ($O_2$ + 10% $O_3$) background pressure was held at $8 \times 10^{-7}$ Torr. Sr was evaporated with a flux of $2 \times 10^{13}$ atoms/cm$^2$s from an effusion cell and shuttered to provide Sr in sequential doses corresponding to the number of Sr atoms in a SrO monolayer. Note that $SrRuO_3$ grown along the $[001]_p$ growth direction can be considered as alternating monolayers of SrO and $RuO_2$. In contrast, Ru was evaporated with a flux of $4 \times 10^{13}$ atoms/cm$^2$s using an electron beam evaporator and supplied continuously during the entire growth. The growth rate was about 0.4 nm/min (1 pseudocubic unit cell per minute) and films were monitored using reflection high-energy electron diffraction (RHEED) along the $[110]_p$ azimuth during growth. RHEED images of the $NdGaO_3$ substrate and $SrRuO_3$ film are shown in Fig. S1. $SrRuO_3$ films exhibit prominent Kikuchi lines, indicating good crystalline perfection, which was found to be a strong indicator of the quality of the photoemission spectra.

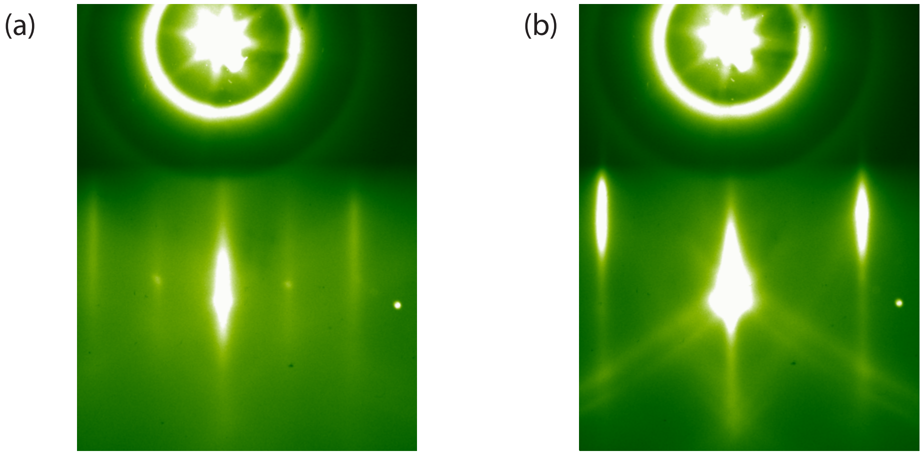


Figure S1: RHEED diffraction images taken along the $[110]_p$ azimuth of (a) the bare $NdGaO_3$ substrate and (b) after the growth of a 20 nm thick $SrRuO_3$ film.

## LOW-ENERGY ELECTRON DIFFRACTION

Following ARPES measurements, films were characterized *in situ* by low-energy electron diffraction (LEED). An exemplary LEED pattern is shown in Fig. S2, taken at normal incidence with a beam energy of 150 eV. The sharp

diffraction peaks indicate a well ordered surface crystal structure. The lowest pseudocubic diffraction beams are indicated in the pattern, and the spots appearing at $\sqrt{2} \times \sqrt{2}$ R45° relative to these are a result of the orthorhombic symmetry of the film.

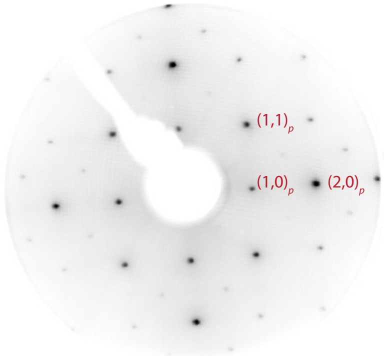


Figure S2: Low-energy electron diffraction (LEED) image of $(001)_p$ $SrRuO_3$, taken with an electron energy of 150 eV.

## X-RAY DIFFRACTION

The phase purity and crystallinity of the $SrRuO_3$ films were characterized *ex situ* by four-circle x-ray diffraction (XRD). $\theta - 2\theta$ and rocking curve in $\omega$ scans are respectively shown in Figs. S3(a) and S3(b). The full width at half maximum of the $\omega$-rocking curve of the $002_p$ film peak was determined to be 22 arcsec, nearly identical to that of the $NdGaO_3$ substrate (18 arcsec), indicating the high crystalline quality of the films.

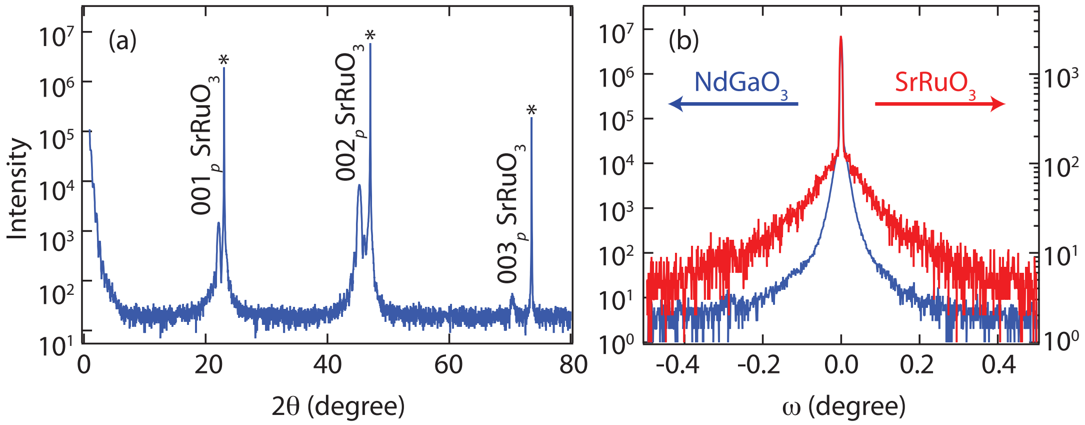


Figure S3: (a) X-ray diffraction $\theta - 2\theta$ scan of a 20 nm thick $SrRuO_3$ film grown on $NdGaO_3$. Substrate peaks are marked with an asterisk (∗). (b) Rocking curve about the $002_p$ peak for both the $SrRuO_3$ film and the underlying $NdGaO_3$ substrate.

* Author to whom correspondence should be addressed: kmshen@cornell.edu
